# Supplementary material for: Single spontaneous photon as a coherent beamsplitter for an atomic matterwave
Source: arXiv:1012.4704 source file (2012-09-27)
Supplement: Supplementary file 1 [file suplementary_information.pdf]

# Supplementary Information

## Experimental details

### Atomic beam preparation

For the experimental implementation a well collimated beam of metastable $^{40}Ar$ atoms is used. The atomic beam is transversally cooled and collimated by a 2D-magneto-optical trap and furthermore collimated by a setup of 2 variable slits, leading to a beam width of 10 $\mu m$ (FWHM) at the position of the first mirror, a spread in momentum distribution of 0.4 photon recoil (HWHM) and a longitudinal velocity of 31 $m/s$. The beam is polarized by applying a Stern-Gerlach magnet configuration.

### Spatially resolved atom detection

Metastable argon atoms allows for spatially resolved single-particle detection using a multichannel plate (MCP) in combination with a resistive anode. By tilting the MCP with respect to the beam axis, the resolution is enhanced to 17 $\mu m$ per Pixel. We evaluated the signal on 3 adjacent pixel. The distance between the experimental chamber and the MCP is 1.05 $m$ so that a momentum transfer of less than a photon recoil can be resolved clearly.

### Electronic structure and detection of coherence

The internal electronic structure of argon allows for a straight forward implementation of spontaneous emission of a single photon (see Fig. 1). Starting in the $1s_5$ $(J = 2, m_j = 0)$ level (Paschen- notation), a laser with a wavelength of 714.903 $nm$ excites the atom to the $2p_4$ level. From there, it can either decay to the ground state – which is not detectable by the MCP, or to two metastable states. A fraction of 96.75 % of all metastable atoms decay by spontaneous emission of a single photon with a wavelength of 795.036 $nm$ to the metastable $1s_3(J = 0)$ state for which the excitation laser is far detuned. Thus reexcitation is strongly suppressed. Although a small fraction (3.25 %) of atoms decay back to the $1s_5$ $(J = 2)$ state, the interaction time of atoms with the excitation laser is chosen to be smaller than the cycle time of Rabi-Oscillations of the cycle $1s_5 \rightarrow 1s_3 \rightarrow 1s_5$ to avoid spontaneous emission of more than one photon. An additional laser at 801.702 $nm$ behind the interaction zone optically quenches the remaining $1s_5$ to the ground state. Thus all detected metastable atoms have undergone a single photon emission event.

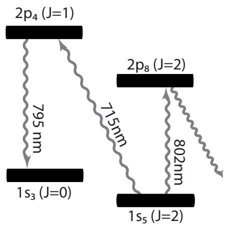


Figure 1: Relevant level scheme of $^{40}Ar$

The Bragg-crystal is conventionally implemented by a standing light wave on a second mirror. The laser is red detuned by 10 $GHz$ to the $1s_3 \leftrightarrow 2p_4$ transition, the same transition where the spontaneous photon is emitted. The width of the standing light wave was chosen to 1.5 $mm$ resulting in a sufficiently large angle acceptance of the Bragg-crystal allowing for compensating small shifts in the original momentum distribution of the atomic beam. The intensity of the Bragg-crystal was adjusted to ensure approximately a 50/50 beam splitting ratio.

### Mirror setup and adjustment

The spontaneous emission takes place in front of a gold coated mirror. It is important to note that for a dielectric mirror the photon reflection is 'deep' in the mirror surface. Thus the effective distance between atom and the reflection point is typically too large to make the effect observable.

The second mirror is mounted on a 3-axis piezo mirror mount so it can be aligned parallel to the first mirror and translated along its normal. Thus the phase of the standing light wave can be shifted with respect to the first mirror and we can scan over a range of more than two interference fringes. Both mirrors are mounted together on a custom made translation/rotation stage, so they can be aligned parallel to the atomic beam. The translation stage transversal to the beam allows for implementing different distances between the beam and the mirror setup without changing the optical alignment.

The intensity of the Bragg crystal and the angle between the atomic beam and the mirrors are adjusted in preliminary experiments by tilting the mirrors in the Bragg angle, shining in only the second standing light wave and probing for Bragg diffraction of about 50%. It was carefully checked that no stray light from the Bragg lattice hits the first mirror.

### Quantification of the intuitive picture

In order to obtain a quantitative prediction within the intuitive picture, we choose the following assumptions. We assign to the atom a size corresponding to the optical absorption cross section $\sigma = 3\lambda^2/2\pi$. The overlap of the atom and the mirror atom in the projection to the observer is a measure for the indistinguishability and thus for the coherence (see Main text, Fig. 1b). This overlap depends on the distance $d$ between atom and mirror and the observation angle $\varphi$ to the mirror normal and can be written as:

$$\begin{aligned} P(d,\varphi) &= \frac{2}{\pi}\left(\arccos\gamma - \gamma\sqrt{1-\gamma^2}\right) \\ \text{with } \gamma &= \frac{d\tan\varphi}{\sqrt{\sigma/\pi}}\,. \end{aligned} \tag{1}$$

The detector integrates over all emission directions located on a spherical calotte. Furthermore the spatial extension of the atomic beam leads to an integration over different atom-mirror distances. Including experimental details as the initial momentum distribution of the atomic beam and the finite angle acceptance of Bragg scattering leads to the prediction for the visibility.

## Quantum mechanical model

The experiment measures the probability $P$ to find an atom after spontaneous emission of a single photon and after diffraction by the Bragg grating within the interval $z_0 \pm \Delta_z/2$, where $\Delta z = 51.6\mu$m (the $z$ direction is perpendicular to the mirror plane). The probability $P$ at $z_0$ depends on the phase $\phi_{\rm B}$ imprinted by the Bragg grating,

$$P = P_0 + \mathcal{A}\cos(\phi_{\rm B} + \phi_0), \tag{2}$$

where $\phi_0$ is an irrelevant constant phase. The calculation of the visibility $V = \mathcal{A}/P_0$ of the interference pattern consists of three steps that we illustrate in the following. First, we determine the quantum state of the atom after the spontaneous emission in front of the mirror. Second, we evaluate the state after the Bragg grating, and the third and final step concerns the detection of the atoms. Throughout the derivation, unit vectors $\vec{\mathbf{v}} = \mathbf{v}/|\mathbf{v}|$ are labeled by an arrow, and operators $\hat{X}$ by a hat.

**Spontaneous emission.** We model the atom by a two-level system with excited state $|e\rangle$, ground state $|g\rangle$, transition frequency $\omega_0$ and transition dipole matrix element $\mathbf{d} = \langle e|\hat{\mathbf{d}}|g\rangle$. The density operator $\hat{\varrho}$ describes the quantum state of the atomic system and contains internal as well as external

degrees of freedom. At $t = 0$, the electromagnetic field is assumed to be in the vacuum state $\hat{\varrho}_{\mathrm{F}}$, and the density operator of the total system is $\hat{\varrho}_{\mathrm{T}} = \hat{\varrho} \otimes \hat{\varrho}_{\mathrm{F}}$. In electric-dipole coupling and rotating-wave approximation, the interaction between the atom and the radiation field is governed by the Hamiltonian

$$\hat{H}_{\mathrm{int}} = -\mathbf{d} \cdot \hat{\mathbf{E}}^{+}(\hat{\mathbf{r}})|e\rangle\langle g| + \mathrm{h.c.}, \tag{3}$$

where $\hat{\mathbf{E}}^{+}(\mathbf{r})$ is the positive frequency part of the electric field operator and $\hat{\mathbf{r}}$ is the position operator. In our model, an absorbing medium with a high reflectivity ($z > 0$) forms a planar interface at $z = 0$ with the vacuum ($z < 0$). For this geometry, the positive frequency part of the electric field operator is given by [1]

$$\hat{\mathbf{E}}^{+}(\mathbf{r}) = \int_{0}^{\infty} \mathrm{d}\omega \hat{\mathbf{E}}^{+}(\mathbf{r}, \omega) + \mathrm{noise}, \tag{4}$$

where

$$\hat{\mathbf{E}}^{+}(\mathbf{r}, \omega) = \frac{i}{A} \sum_{\mathbf{K}} e^{i\mathbf{K}\cdot\mathbf{R}} \alpha_{\mathbf{K}}(\omega) \sum_{\epsilon} U_{\epsilon\mathbf{K}}(z, \omega) \hat{a}_{\epsilon\mathbf{K}}(\omega), \tag{5}$$

$A$ is a quantization surface and $\mathbf{R} = x\vec{\mathbf{e}}_x + y\vec{\mathbf{e}}_y$ is the projection of $\mathbf{r} = (x, y, z)$ onto the $x - y$ plane. Similarly, $\mathbf{K} = k_x\vec{\mathbf{e}}_x + k_y\vec{\mathbf{e}}_y$ denotes the in-plane component of the wave vector $\mathbf{k} = (k_x, k_y, k_z)$, and for a given frequency $\omega$, $|k_z| = \kappa$ is determined by $\kappa(\omega) = \sqrt{\omega^2/c^2 - K^2}$. In Eq. (5), $\hat{a}_{\epsilon\mathbf{K}}$ are photon annihilation operators that obey the usual bosonic commutation relations and $\alpha_{\mathbf{K}}(\omega) = \omega\sqrt{\hbar/4\pi\varepsilon_0 c^2 \kappa(\omega)}$. The index $\epsilon \in \{s, p\}$ labels the two orthogonal modes

$$U_{s\mathbf{K}}(z, \omega) = e^{i\kappa z}\vec{\mathbf{s}} + e^{-i\kappa z} r_s \vec{\mathbf{s}}, \tag{6}$$

$$U_{p\mathbf{K}}(z, \omega) = e^{i\kappa z}\vec{\mathbf{p}}_{+} + e^{-i\kappa z} r_p \vec{\mathbf{p}}_{-}, \tag{7}$$

where $s$ labels the TE (transversal electric) and $p$ the TM (transversal magnetic) mode characterized by the unit vectors

$$\vec{\mathbf{s}} = \vec{\mathbf{K}} \times \vec{\mathbf{e}}_z, \qquad \vec{\mathbf{p}}_{\pm} = (K\vec{\mathbf{e}}_z \mp \kappa\vec{\mathbf{K}})c/\omega. \tag{8}$$

In Eqs. (6) and (7), $r_s$ and $r_p$ are the Fresnel coefficients associated with the reflection of the TE and TM modes at the mirror, respectively. The noise term in Eq. (4) is related to the losses in the half-space $z > 0$ according to the fluctuation-dissipation theorem. In the following, we will neglect this noise term which is justified for a mirror with near-perfect reflectivity.

With standard projection operator techniques [2], we derive a master equation for the reduced density operator $\hat{\varrho}$ of the atom including the center

of mass motion. The momentum components in the mirror plane are traced out such that only the $z$ coordinate of the atomic motion is retained. With $\hat{\varrho}_{gg} = \langle g|\hat{\varrho}|g\rangle$ and $\hat{\varrho}_{ee} = \langle e|\hat{\varrho}|e\rangle$, we find

$$\begin{aligned}
\partial_t \hat{\varrho}_{gg}(t) &= \gamma\frac{3}{8}\Big\{\int_0^1 \mathrm{d}u[r_s^* e^{ik_0u\hat{z}} + e^{-ik_0u\hat{z}}] \\
&\qquad \times \hat{\varrho}_{ee}(t)[r_s e^{-ik_0u\hat{z}} + e^{ik_0u\hat{z}}] \\
&\quad + \int_0^1 \mathrm{d}u u^2[r_p^* e^{ik_0u\hat{z}} - e^{-ik_0u\hat{z}}] \\
&\qquad \times \hat{\varrho}_{ee}(t)[r_p e^{-ik_0u\hat{z}} - e^{ik_0u\hat{z}}]\Big\},
\end{aligned} \tag{9}$$

where $\gamma$ is the full decay rate of the excited state $|e\rangle$ in free space and we assumed that the dipole moment $\mathbf{d}$ is oriented parallel to the mirror. At $t = 0$, we suppose that the atom is prepared in the state $\hat{\varrho}_{gg}(0) = 0$ and $\hat{\varrho}_{ee}(0) = |\psi_0\rangle\langle\psi_0|$, where $|\psi_0\rangle$ is the motional state of the atom before spontaneous emission that we specify below. The quantum state of the atom after spontaneous emission is given by $\hat{\varrho}_{gg}(\infty) = \int_0^\infty \mathrm{d}t \partial_t \hat{\varrho}_{gg}(t)$ and can be obtained from the right-hand side of Eq. (9) if $\hat{\varrho}_{ee}$ is replaced by $\hat{\varrho}_0 = \int_0^\infty \mathrm{d}t \hat{\varrho}_{ee}(t)$. If the mirror were absent, the integral would be given by $\hat{\varrho}_0 = [\hat{\varrho}_{ee}(t=0)/\gamma]$. The mirror gives rise to a position-dependent decay rate that varies on a length scale determined by the wavelength of the optical transition. In order to account for this effect, we take $\hat{\varrho}_0 = (\alpha/\gamma)|\psi_0\rangle\langle\psi_0|$, where $\alpha$ is fixed by the condition $\mathrm{Tr}[\hat{\varrho}_{gg}(\infty)] = 1$. Note that in the present case, the effect of the mirror on $\hat{\varrho}_0$ is small since the spatial extend of $|\psi_0\rangle$ is larger than the wavelength of the transition. The quantum state of the atom after spontaneous emission can then be written as

$$\hat{\varrho}_{gg}(\infty) = \alpha\frac{3}{8}\int_0^1 \mathrm{d}u \left(|\psi_s\rangle\langle\psi_s| + u^2|\psi_p\rangle\langle\psi_p|\right), \tag{10}$$

where

$$|\psi_s\rangle = \left(r_s^* e^{ik_0u\hat{z}} + e^{-ik_0u\hat{z}}\right)|\psi_0\rangle, \tag{11}$$
$$|\psi_p\rangle = \left(-r_p^* e^{ik_0u\hat{z}} + e^{-ik_0u\hat{z}}\right)|\psi_0\rangle. \tag{12}$$

The operators $e^{\pm ik_0u\hat{z}}$ in Eqs. (11) and (12) describe the transverse recoil momentum $\pm\hbar k_0 u$ transferred to the atom by the spontaneously emitted

photon. It follows that $|\psi_s\rangle$ and $|\psi_p\rangle$ represent a coherent superposition of two wave packets that travel at different mean velocities. The state

$$|\psi_0\rangle = \int \mathrm{d}p f(p,d) e^{\frac{i}{\hbar}pd} e^{i\phi_f(p)} |p\rangle \tag{13}$$

describes the motional state of the atom before spontaneous emission and is modeled as a coherent wave packet, where $f(p,d) > 0$ and $[f(p,d)]^2$ represents the initial momentum distribution of the atoms for a given atom-mirror distance $d$. This distribution is inferred from an independent measurement and approximately given by an assymetric Lorentzian. The factor $e^{\frac{i}{\hbar}pd}$ in Eq. (13) ensures that the distance between the center of the wavepacket and the mirror is given by $d$. On the other hand, the phase $\phi_f$ determines the unknown shape of the wave packet in position space and acts as a free parameter that we set to zero in the following.

Note that a mixture of momentum states would not contain any information about the position, since a momentum state is completely delocalized in space. Therefore, the experimentally observed dependence of the interference signal on the atom-mirror distance can only be captured in a model where the atoms are described by a coherent wave packet. Furthermore, the description of the initial atomic state by a pure state, rather than a mixture of pure states, is a good approximation here since the width of the slit collimating the atoms is chosen to be close to the diffraction limit.

**Bragg grating.** The Bragg grating can be described by a unitary operator $U_{\text{bragg}}$ that transfers a momentum state $|p\rangle$ with $p > 0$ into the superposition state

$$U_{\text{bragg}}|p\rangle = \cos\varphi_p |p\rangle + \sin\varphi_p e^{-i\phi_{\mathrm{B}}} |p - 2\hbar k_{\mathrm{L}}\rangle, \tag{14}$$

where $\phi_{\mathrm{B}}$ is a phase factor and $k_{\mathrm{L}}$ is the wave number of the grating. $\cos\varphi_p$ and $\sin\varphi_p$ are the amplitudes of the transmitted and the diffracted components, respectively. These amplitudes are inferred from an independent measurement that characterizes the Bragg grating. Similarly, a momentum state $|q\rangle$ with $q < 0$ becomes

$$U_{\text{bragg}}|q\rangle = \cos\varphi_q |q\rangle - \sin\varphi_q e^{i\phi_{\mathrm{B}}} |q + 2\hbar k_{\mathrm{L}}\rangle. \tag{15}$$

After the diffraction at the Bragg grating, the atomic wave packet undergoes a free time evolution with $U_{\text{free}} = \exp[-i\hat{p}_z^2/(2m\hbar)T]$ for $T = 33.5$ms. The quantum state at the detector is thus given by

$$\hat{\varrho}(\text{detector}) = (U_{\text{free}} U_{\text{bragg}}) \hat{\varrho}_{gg}(\infty) (U_{\text{free}} U_{\text{bragg}})^\dagger, \tag{16}$$

where $\hat{\varrho}_{gg}(\infty)$ is defined in Eq. (10). In order to determine $\hat{\varrho}(\text{detector})$, it suffices to consider the time evolution of the states $|\psi_\epsilon\rangle$ ($\epsilon \in \{s, p\}$) that are defined in Eqs. (11) and (12). The Bragg grating followed by free time evolution transfers $|\psi_\epsilon\rangle$ into a state comprised of four terms,

$$|\tilde{\psi}_\epsilon\rangle = U_{\text{free}} U_{\text{bragg}} |\psi_\epsilon\rangle = |T_\epsilon^-\rangle + e^{-i\phi_{\text{B}}}|D_\epsilon^-\rangle + |T_\epsilon^+\rangle + e^{i\phi_{\text{B}}}|D_\epsilon^+\rangle. \tag{17}$$

In Eqs. (11) and (12), the wave packet described by $e^{-ik_0 u\hat{z}}|\psi_0\rangle$ travels in the negative $z$ direction due to the momentum kick by spontaneous emission. The Bragg grating splits this wave packet into a transmitted and a diffracted part denoted by $|T_\epsilon^-\rangle$ and $|D_\epsilon^+\rangle$, respectively. Here the superscript $\pm$ indicates the propagation direction after the grating. In addition, the wave packet $e^{ik_0 u\hat{z}}|\psi_0\rangle$ travelling in the positive $z$ direction after spontaneous emission is split into a transmitted and a diffracted part denoted by $|T_\epsilon^+\rangle$ and $|D_\epsilon^-\rangle$, respectively.

**Detection.** The detector measures the probability to find an atom in the region $z_0 \pm \Delta_z/2$, where $\Delta z = 51.6\mu\text{m}$. Next we determine the probability $P_\epsilon$ for the detection of an atom in state $|\tilde{\psi}_\epsilon\rangle$ and in an interval around $z_0 < 0$. If $|z_0|$ is sufficiently large, only the wave packets $|T_\epsilon^-\rangle$ and $|D_\epsilon^-\rangle$ overlap such that

$$P_\epsilon = \mathcal{I}_\epsilon + 2\,\text{Re}\mathcal{A}_\epsilon, \tag{18}$$

where Re denotes the real part and

$$\mathcal{I}_\epsilon = \int\limits_{z_0-\Delta_z/2}^{z_0+\Delta_z/2} \mathrm{d}z \left\{ |\langle z|T_\epsilon^-\rangle|^2 + |\langle z|D_\epsilon^-\rangle|^2 \right\}, \tag{19}$$

$$\mathcal{A}_\epsilon = e^{-i\phi_{\text{B}}} \int\limits_{z_0-\Delta_z/2}^{z_0+\Delta_z/2} \mathrm{d}z\, \langle z|D_\epsilon^-\rangle \langle z|T_\epsilon^-\rangle^*. \tag{20}$$

In order to obtain the full detection probability $P$, we have to take the average over the incoherent mixture of states according to Eq. (10),

$$P = \alpha \frac{3}{8} \int\limits_0^1 \mathrm{d}u [P_s(u) + u^2 P_p(u)]. \tag{21}$$

If the latter equation is compared to Eq. (2), it follows that

$$P_0 = \alpha \frac{3}{8} \int\limits_0^1 \mathrm{d}u \left[ \mathcal{I}_s + u^2 \mathcal{I}_p \right], \tag{22}$$

$$\mathcal{A} = \alpha \frac{3}{4} \mathrm{Abs} \left\{ \int\limits_0^1 \mathrm{d}u \left[ \mathcal{A}_s + u^2 \mathcal{A}_p \right] \right\}. \tag{23}$$

Finally, the visibility of the measured interference pattern is given by $V = \mathcal{A}/P_0$.

# References


[1] Di Stefano, O., Savasta, S. & Girlanda, R. Three-dimensional electromagnetic field quantization in absorbing and dispersive bounded dielectrics. Phys. Rev. A **61**, 023803 (2000).

[2] Breuer, H.-P. & Petruccione, F. The Theory of Open Quantum Systems (Oxford University Press, 2006).
